# Supplementary material for: SPT-NRTL: A physics-guided machine learning model to predict thermodynamically consistent activity coefficients
Source: arXiv:2209.04135 ancillary file (2022-09-27)
Supplement: Supplementary file 1 [file SI_SPT_NRTL.pdf]

# Supporting Information to "SPT-NRTL: A physics-guided machine learning model to predict thermodynamically consistent activity coefficients"

Benedikt Winter
ETH Zurich

Clemens Winter
OpenAI

Timm Esper
University of Stuttgart

Johannes Schilling
ETH Zurich

André Bardow
ETH Zurich

September 2, 2022

## Contents

1 **Vocab** 2

2 **Training data distribution** 3

3 **Hyperparameters** 5

4 **Full NRTL Dataset** 6

5 **Molecular groups** 7

# 1 Vocab

Table 1: Vocab used in SPT-NRTL. The vocab contains entries for tokens that are not part of the Brouwer and DDB database and are thus not trained for the models provided. These tokens are not marked as trained. It is not recommended to predict molecules containing untrained tokens without first fine-tuning the model for these tokens as Otherwise very inaccurate predictions are obtained. The model has a embedding matrix of size 128. Thus, the vocab can be extended if more tokens are required in fine-tuning on new datasets without training a new model

| i | Token | Trained | i | Token | Trained |
|---|---|---|---|---|---|
| 0 | $< PAD >$ | x | 34 | P | x |
| 1 | $< SOS >$ | x | 35 | 6 | |
| 2 | $< MOS >$ | x | 36 | I | x |
| 3 | $< EOS >$ | x | 37 | a | x |
| 4 | c | x | 38 | i | x |
| 5 | C | x | 39 | 7 | |
| 6 | ( | x | 40 | e | x |
| 7 | ) | x | 41 | K | x |
| 8 | 1 | x | 42 | 8 | |
| 9 | O | x | 43 | L | |
| 10 | 2 | x | 44 | A | x |
| 11 | = | x | 45 | Z | x |
| 12 | N | x | 46 | g | x |
| 13 | n | x | 47 | M | |
| 14 | 3 | x | 48 | T | x |
| 15 | [ | x | 49 | t | |
| 16 | ] | x | 50 | 9 | |
| 17 | @ | | 51 | p | |
| 18 | H | x | 52 | % | |
| 19 | F | x | 53 | 0 | |
| 20 | - | x | 54 | V | |
| 21 | 4 | | 55 | b | x |
| 22 | S | x | 56 | u | |
| 23 | l | x | 57 | R | |
| 24 | / | | 58 | X | |
| 25 | s | x | 59 | H2O | |
| 26 | o | x | 60 | d | |
| 27 | + | x | 61 | G | x |
| 28 | 5 | | 62 | Y | |
| 29 | # | x | 63 | D | |
| 30 | . | x | 64 | y | |
| 31 | B | x | 65 | W | x |
| 32 | r | x | 66 | | |
| 33 | \ | | | | |

## 2 Training data distribution

In the following the distribution of temperature, concentration and $ln\gamma$ is shown for the Brouwer[Brouwer et al., 2021] and the DDB [Dortmund Datenbank, 2022] dataset. The Brouwer dataset contains 20 870 data points with 349 solvents and 373 solutes in 6416 unique combinations at temperatures ranging from 250 K to 555.6 K (Figure 1 and Figure 2).

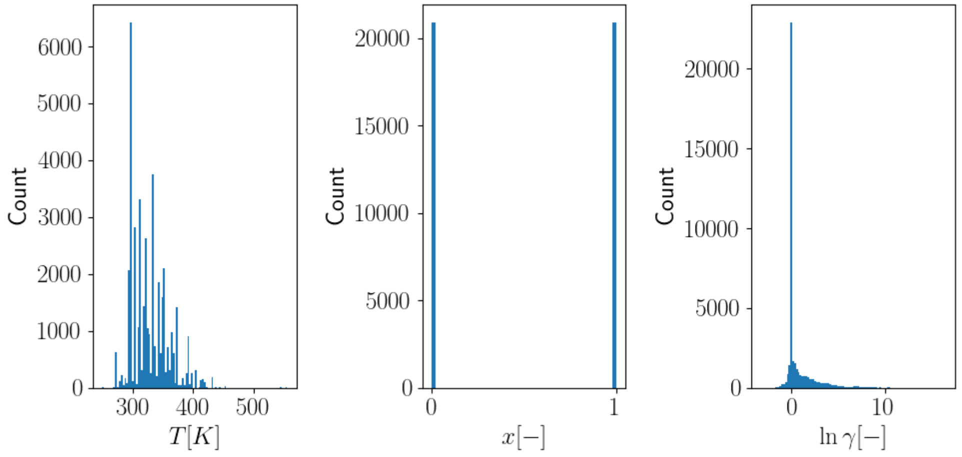


Figure 1: Histograms of the temperature $T$, mole fraction $x$ and $\ln\gamma$ distribution for the Brouwer dataset. For the Brouwer dataset all datapoints have a mole fraction of either 0 or 1

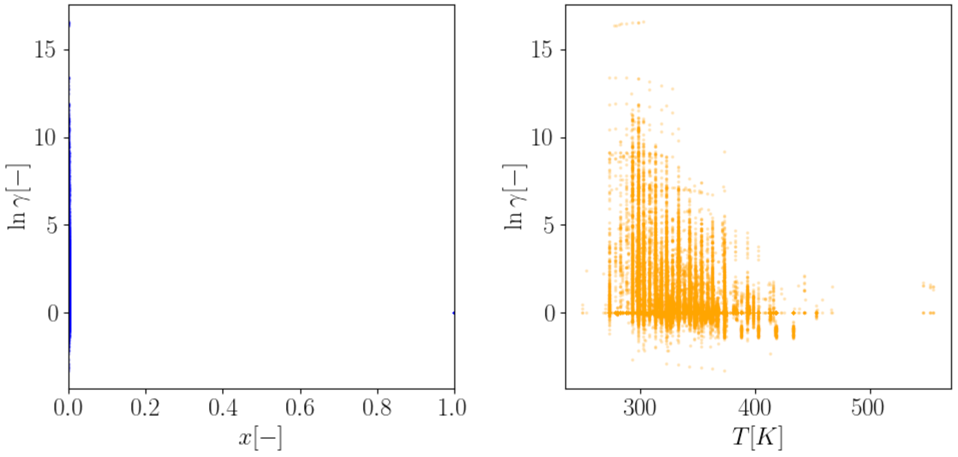


Figure 2: Distribution of $\ln\gamma$ as a function of the mole fraction $x$ and temperature $T$ for the Brouwer dataset.

The considered DDB dataset of concentration-dependent activity coefficients contains 77 053 data points with 506 components in 2302 unique combinations at temperatures between 183.0 K and 973.15 K (Figure 3 and Figure4).

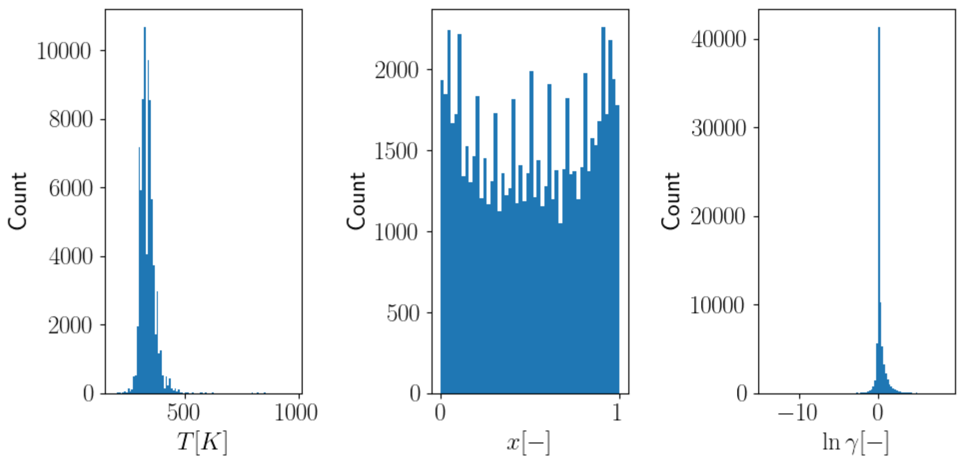


Figure 3: Histograms of the temperature $T$, mole fraction $x$ and $\ln \gamma$ distribution for the DDB dataset.

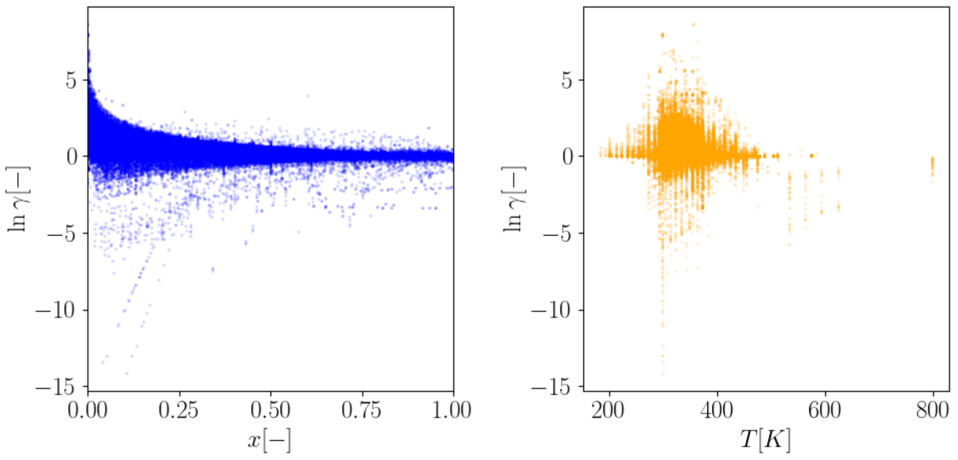


Figure 4: Distribution of $\ln \gamma$ as a function of the mole fraction $x$ and temperature $T$ for the Brouwer dataset.

# 3 Hyperparameters

In Table 2, Table 3 and Table 4 the hyperparameters of the pretrained models are listed. As SPT-NRTL is build up from an SPT model [Winter et al., 2022], the architectural hyperparameters remain the same. The learning rate of the pretraining was manually adjusted to yield good results.

Table 2: Model parameters of the SPT-NRTL model.

| Model parameter | Value |
|---|---|
| Embedding size | 512 |
| Number of attention-heads | 16 |
| Number of transformer blocks | 2 |
| Dropout | 0 |

Table 3: Training parameters for the pretraining of the SPT-NRTL model.

| Model parameter | Value |
|---|---|
| Batch Size | 1024 |
| Maximum learning rate | 1e-5 |
| Epochs | 10 |
| Warm up increase | 10 |
| Weight decay | 0 |

Table 4: Training parameters for the fine-tuning of the SPT-NRTL model.

| Model parameter | Value |
|---|---|
| Batch Size | 256 |
| Maximum learning rate | 1e-4 |
| Epochs | 10 |
| Warm up increase | 100 |
| Weight decay | 0 |

# 4 Full NRTL Dataset

An SPT-NRTL model trained on the full available dataset is used to calculate the NRTL parameters of all combinations of 10 000 molecules, yielding a total of 100 000 000 sets of NRTL parameters. These parameters are available at: https://polybox.ethz.ch/index.php/s/unM7rbgj2FQPFdy

Molecules can be found using the canonical SMILES created by the python package `rdkit` .

# 5 Molecular groups

In Table 5, all molecules within the training set used for fine-tuning are listed with their name, SMILES code and the functional group assigned to it.

Table 5: List of all molecules contained in the Brouwer and DDB dataset with the assigned functional groups.

| Name | SMILES | Group |
|---|---|---|
| acetaldehyde | CC=O | Aldehyde |
| acetamide | CC(N)=O | Nitrate |
| acetonitrile | CC#N | Nitrate |
| propan-2-one | CC(C)=O | Keton |
| ethane-1,2-diamine | NCCN | Nitrate |
| 1,2-dibromoethyne | BrCCBr | Halogene |
| bromoethane | CCBr | Halogene |
| ethane-1,2-diol | OCCO | Alcohol |
| iodoethane | CCI | Halogene |
| ethanol | CCO | Alcohol |
| ethoxyethane | CCOCC | Ether |
| oxirane | C1CO1 | Ether |
| prop-2-en-1-ol | C=CCO | Alcohol |
| formic acid | O=CO | Aliphatic |
| ethyl formate | CCOC=O | Ether |
| aniline | Nc1ccccc1 | Nitrate |
| methoxybenzene | COc1ccccc1 | Ether |
| 2-methylpyridine | Cc1ccccn1 | Nitrate |
| 4,7,7-trimethylbicyclo[3.1.1]hept-3-ene | CC1=CCC2CC1C2(C)C | Aliphatic |
| ethyl acetate | CCOC(C)=O | Multiple |
| butan-2-ol | CCC(C)O | Alcohol |
| butane-2,3-diol | CC(O)C(C)O | Alcohol |
| phenylmethanol | OCc1ccccc1 | Alcohol |
| ethylbenzene | CCc1ccccc1 | Aromat |
| bromobenzene | Brc1ccccc1 | Halogene |
| chlorobenzene | Clc1ccccc1 | Halogene |
| 1,4-dichlorobenzene | Clc1ccc(Cl)cc1 | Halogene |
| benzonitrile | N#Cc1ccccc1 | Nitrate |
| nitrobenzene | O=[N+]([O-])c1ccccc1 | Nitrate |
| benzene | c1ccccc1 | Aromat |
| 7,7-dimethyl-4-methylidenebicyclo[3.1.1]heptane | C=C1CCC2CC1C2(C)C | Aliphatic |
| 1-bromobutane | CCCCBr | Halogene |

| | | |
|---|---|---|
| molecular bromine | BrBr | Other |
| 2-butoxyethanol | CCCCOCCO | Multiple |
| butan-1-ol | CCCCO | Alcohol |
| butan-2-one | CCC(C)=O | Keton |
| butane | CCCC | Aliphatic |
| 1-chloro-2-methylpropane | CC(C)CCl | Halogene |
| N-butan-2-ylidenehydroxylamine | CCC(C)=NO | Nitrate |
| 1-chlorobutane | CCCCCl | Halogene |
| chloroform | ClC(Cl)Cl | Halogene |
| 3-methylphenol | Cc1cccc(O)c1 | Alcohol |
| cyclohexane | C1CCCCC1 | Aliphatic |
| cyclopentane | C1CCCC1 | Aliphatic |
| cyclohexene | C1=CCCCC1 | Aliphatic |
| methylcyclohexane | CC1CCCCC1 | Aliphatic |
| methylcyclopentane | CC1CCCC1 | Aliphatic |
| 1-butoxybutane | CCCCOCCCC | Ether |
| decane | CCCCCCCCCC | Aliphatic |
| n-ethylethanamine | CCNCC | Nitrate |
| butane-2,3-dione | CC(=O)C(C)=O | Keton |
| n,n-dimethylaniline | CN(C)c1ccccc1 | Nitrate |
| 1,1-dichloroethane | CC(Cl)Cl | Halogene |
| 1,2-dichloroethane | ClCCCl | Halogene |
| 1,2-dichloroethene | ClC=CCl | Halogene |
| dichloromethane | ClCCl | Halogene |
| n,n-dimethylformamide | CN(C)C=O | Nitrate |
| dimethoxymethane | COCOC | Ether |
| 2,4-dimethylpentane | CC(C)CC(C)C | Aliphatic |
| 1,4-dioxane | C1COCCO1 | Ether |
| 2,6-dimethylpyridine | Cc1cccc(C)n1 | Nitrate |
| dodecane | CCCCCCCCCCCC | Aliphatic |
| benzaldehyde | O=Cc1ccccc1 | Aldehyde |
| butyl acetate | CCCCOC(C)=O | Multiple |
| methyl acetate | COC(C)=O | Multiple |
| acetic acid | CC(=O)O | Carboxyl |
| furan-2-carbaldehyde | O=Cc1ccco1 | Aldehyde |
| bromane | Br | Other |
| hexane | CCCCCC | Aliphatic |
| fluorane | F | Other |
| heptane | CCCCCCC | Aliphatic |
| hydrazine | NN | Other |

| | | |
|---|---|---|
| 2-methylbutane | CCC(C)C | Aliphatic |
| propan-2-ol | CC(C)O | Alcohol |
| 2-propan-2-yloxypropane | CC(C)OC(C)C | Ether |
| 2,2,4-trimethylpentane | CC(C)CC(C)(C)C | Aliphatic |
| 2-methylbuta-1,3-diene | C=CC(=C)C | Aliphatic |
| iodomethane | CI | Halogene |
| hex-1-ene | C=CCCCC | Aliphatic |
| 2-methylbut-3-yn-2-ol | C#CC(C)(C)O | Alcohol |
| n-ethyl-n-methylethanamine | CCN(C)CC | Nitrate |
| 1-methylnaphthalene | Cc1cccc2ccccc12 | Aromat |
| 2-methylnaphthalene | Cc1ccc2ccccc2c1 | Aromat |
| methanol | CO | Alcohol |
| 2-methylpentane | CCCC(C)C | Aliphatic |
| 3-methylpentane | CCC(C)CC | Aliphatic |
| 2-methoxyethanol | COCCO | Multiple |
| morpholine | C1COCCN1 | Multiple |
| 4-hydroxy-4-methylpentan-2-one | CC(=O)CC(C)(C)O | Multiple |
| butylbenzene | CCCCc1ccccc1 | Aromat |
| 4-methylpentan-2-one | CC(=O)CC(C)C | Keton |
| 3-methylpyridine | Cc1cccnc1 | Nitrate |
| 4-methylpyridine | Cc1ccncc1 | Nitrate |
| 2-methylpropan-1-ol | CC(C)CO | Alcohol |
| prop-1-en-2-ylbenzene | C=C(C)c1ccccc1 | Aromat |
| 3-(1-methylpyrrolidin-2-yl)pyridine | CN1CCCC1c1cccnc1 | Nitrate |
| n,n-dihydroxymethanamine | C[N+](=O)[O-] | Nitrate |
| 1-nitropropane | CCC[N+](=O)[O-] | Nitrate |
| nonan-1-ol | CCCCCCCCCO | Alcohol |
| octane | CCCCCCCC | Aliphatic |
| oct-1-ene | C=CCCCCCC | Aliphatic |
| 2-methylphenol | Cc1ccccc1O | Alcohol |
| 4-methylphenol | Cc1ccc(O)cc1 | Alcohol |
| pentane | CCCCC | Aliphatic |
| pentan-1-ol | CCCCCO | Alcohol |
| pentan-2-one | CCCC(C)=O | Keton |
| phenol | Oc1ccccc1 | Alcohol |
| carbonyl dichloride | O=C(Cl)Cl | Halogene |
| propan-1-ol | CCCO | Alcohol |
| propanoic acid | CCC(=O)O | Carboxyl |
| 2-methyloxirane | CC1CO1 | Ether |
| pyridine | c1ccncc1 | Nitrate |

| | | |
|---|---|---|
| nitric acid | O=[N+]([O-])O | Other |
| chlorane | Cl | Halogene |
| sulfuric acid | O=S(=O)(O)O | Multiple |
| methanedithione | S=C=S | Aliphatic |
| ethenylbenzene | C=Cc1ccccc1 | Aromat |
| methylsulfinylmethane | CS(C)=O | Aliphatic |
| 2-methylpropan-2-ol | CC(C)(C)O | Alcohol |
| tetradecane | CCCCCCCCCCCCCC | Aliphatic |
| 1,2,3,4,4a,5,6,7,8,8a-decahydronaphthalene | C1CCC2CCCCC2C1 | Aliphatic |
| 1,2,3,4-tetrahydronaphthalene | c1ccc2c(c1)CCCC2 | Aromat |
| tetrachloromethane | ClC(Cl)(Cl)Cl | Halogene |
| oxolane | C1CCOC1 | Ether |
| methylbenzene | Cc1ccccc1 | Aromat |
| n,n-diethylethanamine | CCN(CC)CC | Nitrate |
| 1,1,2,2-tetrachloroethene | ClC(Cl)=C(Cl)Cl | Halogene |
| 1,1,1-trichloroethane | CC(Cl)(Cl)Cl | Halogene |
| 1,1,2-trichloroethene | ClC=C(Cl)Cl | Halogene |
| trifluoromethylbenzene | FC(F)(F)c1ccccc1 | Halogene |
| ethenyl acetate | C=COC(C)=O | Multiple |
| oxidane | O | Water |
| 1,3-dimethylbenzene | Cc1cccc(C)c1 | Aromat |
| 1,4-dimethylbenzene | Cc1ccc(C)cc1 | Aromat |
| ethyl-dihydroxyazanium | CC[N+](=O)[O-] | Nitrate |
| cyclopentanol | OC1CCCC1 | Alcohol |
| fluorobenzene | Fc1ccccc1 | Halogene |
| tetrachlorosilane | Cl[Si](Cl)(Cl)Cl | Other |
| tetrachlorotitanium | Cl[Ti](Cl)(Cl)Cl | Other |
| trichloro-hydroxyphosphanium | O=P(Cl)(Cl)Cl | Other |
| trichloro-methylsilane | C[Si](Cl)(Cl)Cl | Other |
| sulfuryl dichloride | O=S(=O)(Cl)Cl | Halogene |
| 1,1,2,2-tetrachloroethane | ClC(Cl)C(Cl)Cl | Halogene |
| tetrachlorostannane | Cl[Sn](Cl)(Cl)Cl | Halogene |
| ethyl propanoate | CCOC(=O)CC | Multiple |
| ammonia | N | Multiple |
| chloroethene | C=CCl | Halogene |
| 1,1,2,2,3,3,4,4,5,5-decafluorocyclopentane | FC1(F)C(F)(F)C(F)(F)C(F)(F)C1(F)F | Halogene |
| 1,1,1,2,2,3,3,4,4,5,5,5-dodecafluoropentane | FC(F)(F)C(F)(F)C(F)(F)C(F)(F)C(F)(F)F | Halogene |
| 2-chloro-2-methylpropane | CC(C)(C)Cl | Halogene |
| 1,1,2-trichloro-1,2,2-trifluoroethane | FC(F)(Cl)C(F)(Cl)Cl | Halogene |
| n,n-dimethylacetamide | CC(=O)N(C)C | Nitrate |

| | | |
|---|---|---|
| acrylonitrile | C=CC#N | Nitrate |
| propane-1,2,3-triol | OCC(O)CO | Alcohol |
| acetyl acetate | CC(=O)OC(C)=O | Multiple |
| 2-methylbut-3-en-2-ol | C=CC(C)(C)O | Alcohol |
| butanoic acid | CCCC(=O)O | Carboxyl |
| propane | CCC | Aliphatic |
| propyl acetate | CCCOC(C)=O | Multiple |
| piperidine | C1CCNCC1 | Nitrate |
| chloro-difluoromethane | FC(F)Cl | Halogene |
| dichloro-difluoromethane | FC(F)(Cl)Cl | Halogene |
| 1,1,2,2,3,3,4,4-octafluorocyclobutane | FC1(F)C(F)(F)C(F)(F)C1(F)F | Halogene |
| cyclohexanone | O=C1CCCCC1 | Keton |
| cyclohexanol | OC1CCCCC1 | Alcohol |
| methyl hexadecanoate | CCCCCCCCCCCCCCCC(=O)OC | Multiple |
| 2-methylbut-2-ene | CC=C(C)C | Aliphatic |
| 3-methylbutan-1-ol | CC(C)CCO | Alcohol |
| hexanoic acid | CCCCCC(=O)O | Carboxyl |
| 2-ethoxyethanol | CCOCCO | Multiple |
| 2,4-dimethylphenol | Cc1ccc(O)c(C)c1 | Alcohol |
| 3,5-dimethylphenol | Cc1cc(C)cc(O)c1 | Alcohol |
| propane-1,2-diol | CC(O)CO | Alcohol |
| thiophene | c1ccsc1 | Aromat |
| 1-methylpyrrolidin-2-one | CN1CCCC1=O | Nitrate |
| pentan-3-one | CCC(=O)CC | Keton |
| 2-methylfuran | Cc1ccco1 | Aromat |
| n-methylacetamide | CNC(C)=O | Nitrate |
| hexan-1-ol | CCCCCCO | Alcohol |
| prop-2-enoic acid | C=CC(=O)O | Carboxyl |
| cyclohexanamine | NC1CCCCC1 | Nitrate |
| methyl benzoate | COC(=O)c1ccccc1 | Multiple |
| methyl 3-methylbenzoate | COC(=O)c1cccc(C)c1 | Multiple |
| 2-methylpropane | CC(C)C | Aliphatic |
| 2-bromo-2-chloro-1,1,1-trifluoroethane | FC(F)(F)C(Cl)Br | Halogene |
| 1,2-dimethylbenzene | Cc1ccccc1C | Aromat |
| 1-chloropropane | CCCCl | Halogene |
| 1-propoxypropane | CCCOCCC | Ether |
| 1-ethoxybutane | CCCCOCC | Ether |
| heptan-1-ol | CCCCCCCO | Alcohol |
| decan-1-ol | CCCCCCCCCCO | Alcohol |
| dodecanoic acid | CCCCCCCCCCCC(=O)O | Carboxyl |

| | | |
|---|---|---|
| buta-1,3-diene | C=CC=C | Aliphatic |
| 2,3-dimethylbutane | CC(C)C(C)C | Aliphatic |
| but-1-ene | C=CCC | Aliphatic |
| propylbenzene | CCCc1ccccc1 | Aromat |
| 1,3-dioxolane | C1COCO1 | Ether |
| cycloheptane | C1CCCCCC1 | Aliphatic |
| nonane | CCCCCCCCC | Aliphatic |
| ethylcyclohexane | CCC1CCCCC1 | Aliphatic |
| ethylsulfanylethane | CCSCC | Aliphatic |
| trimethyl-trimethylsilyloxysilane | C[Si](C)(C)O[Si](C)(C)C | Multiple |
| quinoline | c1ccc2ncccc2c1 | Nitrate |
| 2-(chloromethyl)oxirane | ClCC1CO1 | Multiple |
| chloro-trifluoromethane | FC(F)(F)Cl | Halogene |
| dimethyl carbonate | COC(=O)OC | Ether |
| 2-(2-hydroxyethoxy)ethanol | OCCOCCO | Multiple |
| methyl prop-2-enoate | C=CC(=O)OC | Multiple |
| 1,3,5-trimethylbenzene | Cc1cc(C)cc(C)c1 | Aromat |
| chloromethylbenzene | ClCc1ccccc1 | Halogene |
| phenoxybenzene | c1ccc(Oc2ccccc2)cc1 | Ether |
| 6,6-dimethyl-5-methylidenebicyclo[2.2.1]heptane | C=C1C2CCC(C2)C1(C)C | Aliphatic |
| 1,2,4-trimethylbenzene | Cc1ccc(C)c(C)c1 | Aromat |
| dodecan-1-ol | CCCCCCCCCCCCO | Alcohol |
| thiolane 1,1-dioxide | O=S1(=O)CCCC1 | Aliphatic |
| 1,2-dichloro-1,1,2,2-tetrafluoroethane | FC(F)(Cl)C(F)(F)Cl | Halogene |
| 2,4,4-trimethylpent-1-ene | C=C(C)CC(C)(C)C | Aliphatic |
| methoxymethane | COC | Ether |
| 1,1,1,5-tetrachloropentane | ClCCCCC(Cl)(Cl)Cl | Halogene |
| hept-1-ene | C=CCCCCC | Aliphatic |
| 1,1,2,2,3,3,4,4,5,5,6-undecafluoro-6-(trifluoromethyl)cyclohexane | FC(F)(F)C1(F)C(F)(F)C(F)(F)C(F)(F)C(F)(F)C1(F)F | Halogene |
| 3,3-dimethylbutan-2-one | CC(=O)C(C)(C)C | Keton |
| 2-methylbutan-1-ol | CCC(C)CO | Alcohol |
| 2,2-dimethylpropan-1-ol | CC(C)(C)CO | Alcohol |
| 2-methylbutan-2-ol | CCC(C)(C)O | Alcohol |
| dibromomethane | BrCBr | Halogene |
| 1-chloro-2-methylbenzene | Cc1ccccc1Cl | Halogene |
| ethyl 3-oxobutanoate | CCOC(=O)CC(C)=O | Multiple |
| undecane | CCCCCCCCCCC | Aliphatic |
| oxane | C1CCOCC1 | Ether |

| | | |
|---|---|---|
| 2-methoxy-2-methylpropane | COC(C)(C)C | Ether |
| cyclopentene | C1=CCCC1 | Aliphatic |
| 2-chlorobutane | CCC(C)Cl | Halogene |
| 2-chloro-1,1,1,2-tetrafluoroethane | FC(Cl)C(F)(F)F | Halogene |
| prop-1-ene | C=CC | Aliphatic |
| 2,2,2-trifluoroethanol | OCC(F)(F)F | Multiple |
| NA | ClCBr | Halogene |
| bromo-difluoromethane | FC(F)Br | Halogene |
| ethyl octadecanoate | CCCCCCCCCCCCCCCCCC(=O)OCC | Multiple |
| pentan-1-amine | CCCCCN | Nitrate |
| methyldisulfanylmethane | CSSC | Aliphatic |
| 1-chloro-1,1-difluoroethane | CC(F)(F)Cl | Halogene |
| 2-ethyloxirane | CCC1CO1 | Ether |
| 3,7-dimethylocta-1,6-dien-3-ol | C=CC(C)(O)CCC=C(C)C | Alcohol |
| tetrachlorogermane | Cl[Ge](Cl)(Cl)Cl | Halogene |
| 1,1,1,2-tetrafluoroethane | FCC(F)(F)F | Halogene |
| bromine trifluoride | FBr(F)F | Other |
| 1,1,1,2,2-pentafluoro-2-iodoethane | FC(F)(F)C(F)(F)I | Halogene |
| 1-methoxypropan-2-ol | COCC(C)O | Multiple |
| tetraethylgermane | CC[Ge](CC)(CC)CC | Aliphatic |
| lead chloride | Cl[Pb]Cl | Other |
| sodium nitrate | O=[N+]([O-])[O-].[Na+] | Other |
| potassium nitrate | O=[N+]([O-])[O-].[K+] | Other |
| diethylmercury | CC[Hg]CC | Aliphatic |
| 2-chloro-3,3,3-trifluoroprop-1-ene | C=C(Cl)C(F)(F)F | Halogene |
| methane | C | Aliphatic |
| ethane | CC | Aliphatic |
| 2,2-dimethylpropane | CC(C)(C)C | Aliphatic |
| 2,2-dimethylbutane | CCC(C)(C)C | Aliphatic |
| 2-methylhexane | CCCCC(C)C | Aliphatic |
| 3-methylhexane | CCCC(C)CC | Aliphatic |
| 2,2-dimethylpentane | CCCC(C)(C)C | Aliphatic |
| 2,3-dimethylpentane | CCC(C)C(C)C | Aliphatic |
| 3,3-dimethylpentane | CCC(C)(C)CC | Aliphatic |
| 2,2,3-trimethylbutane | CC(C)C(C)(C)C | Aliphatic |
| 3-ethylpentane | CCC(CC)CC | Aliphatic |
| cyclooctane | C1CCCCCCC1 | Aliphatic |
| 2-methylheptane | CCCCCC(C)C | Aliphatic |
| 3-methylheptane | CCCCC(C)CC | Aliphatic |
| 4-methylheptane | CCCC(C)CCC | Aliphatic |

| | | |
|---|---|---|
| 2,3,4-trimethylpentane | CC(C)C(C)C(C)C | Aliphatic |
| 2,2-dimethylhexane | CCCCC(C)(C)C | Aliphatic |
| 2,4-dimethylhexane | CCC(C)CC(C)C | Aliphatic |
| 3,4-dimethylhexane | CCC(C)C(C)CC | Aliphatic |
| 2,5-dimethylhexane | CC(C)CCC(C)C | Aliphatic |
| 2,2,3,3-tetramethylbutane | CC(C)(C)C(C)(C)C | Aliphatic |
| 1,4-dimethylcyclohexane | CC1CCC(C)CC1 | Aliphatic |
| 1,2-dimethylcyclohexane | CC1CCCCC1C | Aliphatic |
| 2,2,4-trimethylhexane | CCC(C)CC(C)(C)C | Aliphatic |
| 2,3,3-trimethylhexane | CCCC(C)(C)C(C)C | Aliphatic |
| 2,3,3a,4,5,6,7,7a-octahydro-1h-indene | C1CCC2CCCC2C1 | Aliphatic |
| cyclodecane | C1CCCCCCCCC1 | Aliphatic |
| tridecane | CCCCCCCCCCCCC | Aliphatic |
| cumene | CC(C)c1ccccc1 | Aromat |
| tert-butylbenzene | CC(C)(C)c1ccccc1 | Aromat |
| pentylbenzene | CCCCCc1ccccc1 | Aromat |
| hexylbenzene | CCCCCCc1ccccc1 | Aromat |
| 1,4-dimethyl-7-propan-2-ylazulene | Cc1ccc(C(C)C)cc2c(C)ccc1-2 | Aromat |
| pent-1-ene | C=CCCC | Aliphatic |
| pent-2-ene | CC=CCC | Aliphatic |
| 3-methylpent-1-ene | C=CC(C)CC | Aliphatic |
| cyclopenta-1,3-diene | C1=CCC=C1 | Aliphatic |
| 3-methylbut-1-ene | C=CC(C)C | Aliphatic |
| penta-1,4-diene | C=CCC=C | Aliphatic |
| penta-1,3-diene | C=CC=CC | Aliphatic |
| hex-2-ene | CC=CCCC | Aliphatic |
| 2,3-dimethylbut-2-ene | CC(C)=C(C)C | Aliphatic |
| hex-3-ene | CCC=CCC | Aliphatic |
| 2-methylpent-1-ene | C=C(C)CCC | Aliphatic |
| 2-methylpent-2-ene | CCC=C(C)C | Aliphatic |
| 4-methylpent-1-ene | C=CCC(C)C | Aliphatic |
| hexa-1,5-diene | C=CCCC=C | Aliphatic |
| hexa-1,4-diene | C=CCC=CC | Aliphatic |
| hexa-1,3-diene | C=CC=CCC | Aliphatic |
| 3-methylcyclopentene | CC1C=CCC1 | Aliphatic |
| cyclohexa-1,3-diene | C1=CCCC=C1 | Aliphatic |
| cyclohexa-1,4-diene | C1=CCC=CC1 | Aliphatic |
| cycloheptene | C1=CCCCCC1 | Aliphatic |
| 4-ethenylcyclohexene | C=CC1CC=CCC1 | Aliphatic |
| hepta-1,6-diene | C=CCCCC=C | Aliphatic |

| | | |
|---|---|---|
| 1-cyclooctene | C1=CCCCCCC1 | Aliphatic |
| octa-1,7-diene | C=CCCCCC=C | Aliphatic |
| non-1-ene | C=CCCCCCCC | Aliphatic |
| 1-methyl-4-prop-1-en-2-ylcyclohexene | C=C(C)C1CC=C(C)CC1 | Aliphatic |
| dec-1-ene | C=CCCCCCCCC | Aliphatic |
| 3,7,7-trimethylbicyclo[3.1.1]hept-3-ene | CC1=CC2CC(C1)C2(C)C | Aliphatic |
| undec-1-ene | C=CCCCCCCCCC | Aliphatic |
| dodec-1-ene | C=CCCCCCCCCCC | Aliphatic |
| tetradec-1-ene | C=CCCCCCCCCCCCC | Aliphatic |
| pent-1-yne | C#CCCC | Aliphatic |
| hex-1-yne | C#CCCCC | Aliphatic |
| hex-2-yne | CC#CCCC | Aliphatic |
| hex-3-yne | CCC#CCC | Aliphatic |
| hept-1-yne | C#CCCCCC | Aliphatic |
| oct-1-yne | C#CCCCCCC | Aliphatic |
| oct-4-yne | CCCC#CCCC | Aliphatic |
| non-1-yne | C#CCCCCCCC | Aliphatic |
| pent-1-yne | C#CCCCCCCCC | Aliphatic |
| pentan-2-ol | CCCC(C)O | Alcohol |
| pentan-3-ol | CCC(O)CC | Alcohol |
| 3-methylbutan-2-ol | CC(C)C(C)O | Alcohol |
| hexan-2-ol | CCCCC(C)O | Alcohol |
| octan-1-ol | CCCCCCCCO | Alcohol |
| 2-phenylethanol | OCCc1ccccc1 | Alcohol |
| propane-1,3-diol | OCCCO | Alcohol |
| butane-1,2-diol | CCC(O)CO | Alcohol |
| butane-1,3-diol | CC(O)CCO | Alcohol |
| butane-1,4-diol | OCCCCO | Alcohol |
| methyl formate | COC=O | Ether |
| methyl propanoate | CCC(=O)OC | Multiple |
| methyl butanoate | CCCC(=O)OC | Multiple |
| methyl pentanoate | CCCCC(=O)OC | Multiple |
| methyl hexanoate | CCCCCC(=O)OC | Multiple |
| ethyl butanoate | CCCC(=O)OCC | Multiple |
| propyl formate | CCCOC=O | Ether |
| propan-2-yl acetate | CC(=O)OC(C)C | Multiple |
| butyl formate | CCCCOC=O | Ether |
| pentyl acetate | CCCCCOC(C)=O | Multiple |
| hexyl acetate | CCCCCCOC(C)=O | Multiple |
| diethyl hexanedioate | CCOC(=O)CCCCC(=O)OCC | Multiple |

| | | |
|---|---|---|
| trimethoxymethane | COC(OC)OC | Ether |
| 2-ethoxy-2-methylpropane | CCOC(C)(C)C | Ether |
| 2-methyl-2-propan-2-yloxypropane | CC(C)OC(C)(C)C | Ether |
| 2-methoxy-2-methylbutane | CCC(C)(C)OC | Ether |
| 2-ethoxy-2-methylbutane | CCOC(C)(C)CC | Ether |
| 2-methoxy-2-methylheptane | CCCCCC(C)(C)OC | Ether |
| furan | c1ccoc1 | Aromat |
| 2,5-dimethylfuran | Cc1ccc(C)o1 | Aromat |
| ethoxybenzene | CCOc1ccccc1 | Ether |
| 1,2-dimethoxyethane | COCCOC | Ether |
| 1-methoxy-2-(2-methoxyethoxy)ethane | COCCOCCOC | Ether |
| 1,3,5-trioxane | C1OCOCO1 | Ether |
| 3-methylbutan-2-one | CC(=O)C(C)C | Keton |
| cyclopentanone | O=C1CCCC1 | Keton |
| pentane-2,4-dione | CC(=O)CC(C)=O | Keton |
| hexan-2-one | CCCCC(C)=O | Keton |
| hexan-3-one | CCCC(=O)CC | Keton |
| heptan-2-one | CCCCCC(C)=O | Keton |
| heptan-4-one | CCCC(=O)CCC | Keton |
| octan-2-one | CCCCCCC(C)=O | Keton |
| nonan-2-one | CCCCCCCC(C)=O | Keton |
| but-3-en-2-one | C=CC(C)=O | Keton |
| formaldehyde | C=O | Aliphatic |
| propanal | CCC=O | Aldehyde |
| butanal | CCCC=O | Aldehyde |
| 2-methylpropanal | CC(C)C=O | Aldehyde |
| pentanal | CCCCC=O | Aldehyde |
| 2-methylbutanal | CCC(C)C=O | Aldehyde |
| 3-methylbutanal | CC(C)CC=O | Aldehyde |
| hexanal | CCCCCC=O | Aldehyde |
| octanal | CCCCCCCC=O | Aldehyde |
| 2-phenylacetaldehyde | O=CCc1ccccc1 | Aldehyde |
| chloroethane | CCCl | Halogene |
| 2-chloropropane | CC(C)Cl | Halogene |
| 1-chloropentane | CCCCCCl | Halogene |
| 1-chlorohexane | CCCCCCCl | Halogene |
| 1-chloroheptane | CCCCCCCCl | Halogene |
| 1-chlorooctane | CCCCCCCCCl | Halogene |
| 1-chlorononane | CCCCCCCCCCl | Halogene |
| 1-chlorodecane | CCCCCCCCCCCl | Halogene |

| | | |
|---|---|---|
| 1-chloroundecane | CCCCCCCCCCCCl | Halogene |
| 1,2-dichloropropane | CC(Cl)CCl | Halogene |
| 1,3-dichloropropane | ClCCCCl | Halogene |
| 1,1,2-trichloroethane | ClCC(Cl)Cl | Halogene |
| 1,1,1,2-tetrachloroethane | ClCC(Cl)(Cl)Cl | Halogene |
| 1,2,4-trichlorobenzene | Clc1ccc(Cl)c(Cl)c1 | Halogene |
| 1,2-dichlorobenzene | Clc1ccccc1Cl | Halogene |
| 1,3-dichlorobenzene | Clc1cccc(Cl)c1 | Halogene |
| 1,1-dichloroethene | C=C(Cl)Cl | Halogene |
| 1,3-dichloropropene | ClC=CCCl | Halogene |
| 4-chloro-2-methoxyphenol | COc1cc(Cl)ccc1O | Multiple |
| 3-chloro-4-hydroxy-5-methoxybenzaldehyde | COc1cc(C=O)cc(Cl)c1O | Multiple |
| 1-bromopropane | CCCBr | Halogene |
| 2-bromopropane | CC(C)Br | Halogene |
| 2-bromobutane | CCC(C)Br | Halogene |
| 1-bromopentane | CCCCCBr | Halogene |
| 1-bromohexane | CCCCCCBr | Halogene |
| 1-bromoheptane | CCCCCCCBr | Halogene |
| 1-bromooctane | CCCCCCCCBr | Halogene |
| 1-bromononane | CCCCCCCCCBr | Halogene |
| 1-bromodecane | CCCCCCCCCCBr | Halogene |
| bromoform | BrC(Br)Br | Halogene |
| 1,1,2,2-tetrabromoethane | BrC(Br)C(Br)Br | Halogene |
| bromo-dichloromethane | ClC(Cl)Br | Halogene |
| bromo-trichloromethane | ClC(Cl)(Cl)Br | Halogene |
| dibromo-chloromethane | ClC(Br)Br | Halogene |
| 1-bromo-2-chloroethyne | ClCCBr | Halogene |
| propionitrile | CCC#N | Nitrate |
| NA | CCCC#N | Nitrate |
| isopropyl cyanide | CC(C)C#N | Nitrate |
| NA | CCCCC#N | Nitrate |
| NA | CCCCCC#N | Nitrate |
| 4-methoxybenzonitrile | COc1ccc(C#N)cc1 | Multiple |
| 2-nitropropane | CC(C)[N+](=O)[O-] | Nitrate |
| 1-nitrobutane | CCCC[N+](=O)[O-] | Nitrate |
| 1-methyl-2-nitrobenzene | Cc1ccccc1[N+](=O)[O-] | Nitrate |
| 1-methyl-3-nitrobenzene | Cc1cccc([N+](=O)[O-])c1 | Nitrate |
| n,n-dihydroxy-4-methylaniline | Cc1ccc([N+](=O)[O-])cc1 | Nitrate |
| 1-fluoropentane | CCCCCF | Halogene |

| | | |
|---|---|---|
| 1-fluorohexane | CCCCCCF | Halogene |
| 1-fluoroheptane | CCCCCCCF | Halogene |
| 1-fluorooctane | CCCCCCCCF | Halogene |
| 1-fluorononane | CCCCCCCCCF | Halogene |
| 1,1-difluoroethane | CC(F)F | Halogene |
| 1,1,1,2,2,3,3,4,4,5,5,6,6,6-tetradecafluorohexane | FC(F)(F)C(F)(F)C(F)(F)C(F)(F)C(F)(F)C(F)(F)F | Halogene |
| 1,1,1,2,2,3,3,4,4,5,5,6,6,7,7,7-hexadecafluoroheptane | FC(F)(F)C(F)(F)C(F)(F)C(F)(F)C(F)(F)C(F)(F)C(F)(F)F | Halogene |
| 1,1,1-trifluorodecane | CCCCCCCCCC(F)(F)F | Halogene |
| 1,2,3,4,5,6-hexafluorobenzene | Fc1c(F)c(F)c(F)c(F)c1F | Halogene |
| 1,1,2,2-tetrachloro-1,2-difluoroethane | FC(Cl)(Cl)C(F)(Cl)Cl | Halogene |
| 1-iodopropane | CCCI | Halogene |
| 2-iodopropane | CC(C)I | Halogene |
| 1-iodobutane | CCCCI | Halogene |
| 1-iodopentane | CCCCCI | Halogene |
| 1-iodohexane | CCCCCCI | Halogene |
| 1-iodoheptane | CCCCCCCI | Halogene |
| 1-iodooctane | CCCCCCCCI | Halogene |
| 1-iodononane | CCCCCCCCCI | Halogene |
| iodobenzene | Ic1ccccc1 | Halogene |
| ethanamine | CCN | Nitrate |
| propan-1-amine | CCCN | Nitrate |
| butan-1-amine | CCCCN | Nitrate |
| hexan-1-amine | CCCCCCN | Nitrate |
| n-propylpropan-1-amine | CCCNCCC | Nitrate |
| n-propan-2-ylpropan-2-amine | CC(C)NC(C)C | Nitrate |
| propane-1,3-diamine | NCCCN | Nitrate |
| 2-aminoethanol | NCCO | Multiple |
| ethyl nitrate | CCO[N+](=O)[O-] | Nitrate |
| propyl nitrate | CCCO[N+](=O)[O-] | Nitrate |
| butyl nitrite | CCCCON=O | Nitrate |
| pentyl nitrite | CCCCCON=O | Nitrate |
| hexyl nitrate | CCCCCCO[N+](=O)[O-] | Nitrate |
| heptyl nitrate | CCCCCCCO[N+](=O)[O-] | Nitrate |
| octyl nitrate | CCCCCCCCO[N+](=O)[O-] | Nitrate |
| propane-1-thiol | CCCS | Aliphatic |
| propane-2-thiol | CC(C)S | Aliphatic |
| butane-1-thiol | CCCCS | Aliphatic |
| methylsulfanylmethane | CSC | Aliphatic |

| | | |
|---|---|---|
| thiolane | C1CCSC1 | Aliphatic |
| trimethyl phosphite | COP(OC)OC | Multiple |
| hydroxy-trimethoxyphosphanium | COP(=O)(OC)OC | Multiple |
| tributoxy-hydroxyphosphanium | CCCCOP(=O)(OCCCC)OCCCC | Multiple |
| hexadecane | CCCCCCCCCCCCCCCC | Aliphatic |
| n-methylpropanamide | CCC(=O)NC | Nitrate |
| n-methylmethanesulfonamide | CNS(C)(=O)=O | Nitrate |
| n-ethylacetamide | CCNC(C)=O | Nitrate |
| n-methylformamide | CNC=O | Nitrate |
| n,n-dimethylpropanamide | CCC(=O)N(C)C | Nitrate |
| morpholine-4-carbaldehyde | O=CN1CCOCC1 | Multiple |
| n,n-dibutylformamide | CCCCN(C=O)CCCC | Nitrate |
| 1-(2-methoxyethoxy)-2-[2-(2-methoxyethoxy)ethoxy]ethane | COCCOCCOCCOCCOC | Ether |
| 2-[2-[2-(2-methoxyethoxy)ethoxy]ethoxy]-2-methylpropane | COCCOCCOCCOC(C)(C)C | Ether |
| 1-[2-[2-(2-butoxyethoxy)ethoxy]ethoxy]butane | CCCCOCCOCCOCCOCCCC | Ether |
| 1-[2-[2-(2-butoxyethoxy)ethoxy]ethoxy]-4,4-dimethylpentane | CCCCOCCOCCOCCOCCCC(C)(C)C | Ether |
| 1-[2-(2-butoxyethoxy)ethoxy]butane | CCCCOCCOCCOCCCC | Ether |
| n-ethylformamide | CCNC=O | Nitrate |
| 2-[2-(2-hydroxyethoxy)ethoxy]ethanol | OCCOCCOCCO | Multiple |
| 2,6,10,15,19,23-hexamethyltetracosane | CC(C)CCCC(C)CCCC(C)CCCCC(C)CCCC(C)CCCC(C)C | Aliphatic |
| pentadecanenitrile | CCCCCCCCCCCCCCC#N | Nitrate |
| 1-phenylethanone | CC(=O)c1ccccc1 | Keton |
| oxolan-2-one | O=C1CCCO1 | Multiple |
| n-bis(dimethylamino)phosphoryl-n-methylmethanamine | CN(C)P(=O)(N(C)C)N(C)C | Other |
| 1,1,1,3,3,3-hexafluoropropan-2-ol | OC(C(F)(F)F)C(F)(F)F | Multiple |
| 1,1,1,2,2,3,3,4,4,5,5,6,6,7,7,8,8,8-octadecafluorooctane | FC(F)(F)C(F)(F)C(F)(F)C(F)(F)C(F)(F)C(F)(F)C(F)(F)C(F)(F)F | Halogene |
| 4-methyl-1,3-dioxolan-2-one | CC1COC(=O)O1 | Ether |
| pyrrolidin-2-one | O=C1CCCN1 | Nitrate |
| 1-methylpiperidin-2-one | CN1CCCCC1=O | Nitrate |
| nonadecan-10-one | CCCCCCCCCC(=O)CCCCCCCCC | Keton |
| furan-2-ylmethanol | OCc1ccco1 | Alcohol |
| n,n-diethylacetamide | CCN(CC)C(C)=O | Nitrate |
| diethyl benzene-1,2-dicarboxylate | CCOC(=O)c1ccccc1C(=O)OCC | Multiple |
| 1-ethylpyrrolidin-2-one | CCN1CCCC1=O | Nitrate |

| | | |
|---|---|---|
| 1,5-dimethylpyrrolidin-2-one | CC1CCC(=O)N1C | Nitrate |
| ethyl benzoate | CCOC(=O)c1ccccc1 | Multiple |
| oxepan-2-one | O=C1CCCCCO1 | Multiple |
| octadecan-1-ol | CCCCCCCCCCCCCCCCCCO | Alcohol |
| icosan-1-ol | CCCCCCCCCCCCCCCCCCCCO | Alcohol |
| tetracosane | CCCCCCCCCCCCCCCCCCCCCCCC | Aliphatic |
| hexadec-1-ene | C=CCCCCCCCCCCCCCC | Aliphatic |
| octadec-1-ene | C=CCCCCCCCCCCCCCCCC | Aliphatic |
| 1-chlorohexadecane | CCCCCCCCCCCCCCCCCl | Halogene |
| 1-chlorooctadecane | CCCCCCCCCCCCCCCCCCCl | Halogene |
| tetradecan-1-ol | CCCCCCCCCCCCCCO | Alcohol |
| dodecan-2-one | CCCCCCCCCCC(C)=O | Keton |
| heptadecan-9-one | CCCCCCCCC(=O)CCCCCCCC | Keton |
| dinonyl benzene-1,2-dicarboxylate | CCCCCCCCCOC(=O)<br>c1ccccc1C(=O)OCCCCCCCCC | Multiple |
| decylbenzene | CCCCCCCCCCc1ccccc1 | Aromat |
| dodecylbenzene | CCCCCCCCCCCCc1ccccc1 | Aromat |
| tetradecylbenzene | CCCCCCCCCCCCCCc1ccccc1 | Aromat |
| pentadecylbenzene | CCCCCCCCCCCCCCCc1ccccc1 | Aromat |
| nonadecylbenzene | CCCCCCCCCCCCCCCCCCCc1ccccc1 | Aromat |
| hexanedinitrile | N#CCCCCC#N | Nitrate |
| 2-methylpentanedinitrile | CC(C#N)CCC#N | Nitrate |
| 2-phenylacetonitrile | N#CCc1ccccc1 | Nitrate |
| 1-cyclohexylpropan-2-one | CC(=O)CC1CCCCC1 | Keton |
| 1-phenylpropan-2-one | CC(=O)Cc1ccccc1 | Keton |
| 4-phenylbutan-2-one | CC(=O)CCc1ccccc1 | Keton |
| 1h-indene | C1=Cc2ccccc2C1 | Aromat |
| 1-chloronaphthalene | Clc1cccc2ccccc12 | Halogene |
| octane-1,8-diamine | NCCCCCCCCN | Nitrate |
| decane-1,10-diamine | NCCCCCCCCCCN | Nitrate |
| dodecane-1,12-diamine | NCCCCCCCCCCCCN | Nitrate |
| tris(2-ethylhexyl) phosphate | CCCCC(CC)COP(=O)(OCC(CC)<br>CCCC)OCC(CC)CCCC | Multiple |
| isoquinoline | c1ccc2cnccc2c1 | Nitrate |
| 2-methylquinoline | Cc1ccc2ccccc2n1 | Nitrate |
| 4-methylquinoline | Cc1ccnc2ccccc12 | Nitrate |
| hexadecanoic acid | CCCCCCCCCCCCCCCC(=O)O | Carboxyl |
| decanedioic acid | O=C(O)CCCCCCCCC(=O)O | Carboxyl |
| heptanedioic acid | O=C(O)CCCCCC(=O)O | Carboxyl |
| octadecane | CCCCCCCCCCCCCCCCCC | Aliphatic |

| | | |
|---|---|---|
| icosane | CCCCCCCCCCCCCCCCCCCC | Aliphatic |
| hexadecan-1-ol | CCCCCCCCCCCCCCCCO | Alcohol |
| n,n-dimethyltetradecanamide | CCCCCCCCCCCCCC(=O)N(C)C | Nitrate |
| dibutyl 3,4,5,6-tetrachlorobenzene-1,2-dicarboxylate | CCCCOC(=O)c1c(Cl)c(Cl)c(Cl)c(Cl)c1C(=O)OCCCC | Multiple |
| dibutyl benzene-1,2-dicarboxylate | CCCCOC(=O)c1ccccc1C(=O)OCCCC | Multiple |
| docosane | CCCCCCCCCCCCCCCCCCCCCC | Aliphatic |
| octacosane | CCCCCCCCCCCCCCCC CCCCCCCCCCCC | Aliphatic |
| triacontane | CCCCCCCCCCCCCCCC CCCCCCCCCCCCCC | Aliphatic |
| dotriacontane | CCCCCCCCCCCCCC CCCCCCCCCCCCCCCCCC | Aliphatic |
| tetratriacontane | CCCCCCCCCCCC CCCCCCCCCCCCCCCCCCCCCC | Aliphatic |
| hexatriacontane | CCCCCCCCCCCCCCC CCCCCCCCCCCCCCCCCCCCC | Aliphatic |
| 2,2,4,4,6,6,8,8-octamethyl-1,3,5,7,2,4,6,8-tetraoxatetrasilocane | C[Si]1(C)O[Si](C)(C)O[Si](C)(C)O[Si](C)(C)O1 | Multiple |
| bis(2-methylpropyl)benzene-1,2-dicarboxylate | CC(C)COC(=O)c1ccccc1C(=O)OCC(C)C | Multiple |
| bis(2-ethylhexyl)benzene-1,2-dicarboxylate | CCCCC(CC)COC(=O)c1ccccc1C(=O)OCC(CC)CCCC | Multiple |
| bis(8-methylnonyl)benzene-1,2-dicarboxylate | CC(C)CCCCCCCOC(=O)c1ccccc1C(=O)OCCCCCCCC(C)C | Multiple |
| o1-butyl o2-(phenylmethyl)benzene-1,2-dicarboxylate | CCCCOC(=O)c1ccccc1C(=O)OCc1ccccc1 | Multiple |
| o2-butyl o1-(2-ethylhexyl)benzene-1,2-dicarboxylate | CCCCOC(=O)c1ccccc1C(=O)OCC(CC)CCCC | Multiple |
| hexane-1,6-diol | OCCCCCCO | Alcohol |
| nonane-1,9-diol | OCCCCCCCCCO | Alcohol |
| hexane-1,6-dithiol | SCCCCCCS | Aliphatic |
| dodecanedinitrile | N#CCCCCCCCCCCCC#N | Nitrate |
| tetrapentylstannane | CCCCC[Sn](CCCCC)(CCCCC)CCCCC | Aliphatic |
| tetraoctylstannane | CCCCCCCC[Sn](CCCCCCCC)(CCCCCCCC)CCCCCCCC | Aliphatic |
| furan-2-ylmethanamine | NCc1ccco1 | Nitrate |
| oxolan-2-ylmethanol | OCC1CCCO1 | Multiple |
| n,n-diethyldodecanamide | CCCCCCCCCCCC(=O)N(CC)CC | Nitrate |
| n-butylbenzamide | CCCCNC(=O)c1ccccc1 | Nitrate |

| | | |
|---|---|---|
| 1,3-dimethylimidazolidin-2-one | CN1CCN(C)C1=O | Nitrate |
| octadecylbenzene | CCCCCCCCCCCCCCCCCCc1ccccc1 | Aromat |
| decylcyclohexane | CCCCCCCCCCC1CCCCC1 | Aliphatic |
| tetradecylcyclohexane | CCCCCCCCCCCCCCC1CCCCC1 | Aliphatic |
| octadecylcyclohexane | CCCCCCCCCCCCCCCCCCC1CCCCC1 | Aliphatic |
| 19,24-dioctadecyldotetracontane | CCCCCCCCCCCCCCCCCCC (CCCCCCCCCCCCCCCCCC) CCCCC(CCCCCCCCCCCCCCCCCC) CCCCCCCCCCCCCCCCCC | Aliphatic |
| cycloheptanol | OC1CCCCCC1 | Alcohol |
| 3-(2-cyanoethoxy)propanenitrile | N#CCCOCCC#N | Multiple |
| 3-(2-cyanoethylsulfanyl)propanenitrile | N#CCCSCCC#N | Nitrate |
| 3-(2-cyanoethylamino)propanenitrile | N#CCCNCCC#N | Nitrate |
| 5-ethyl-2-(2-ethylhexyl)-2-methylnonanamide | CCCCC(CC)CCC(C)(CC (CC)CCCC)C(N)=O | Nitrate |
| 1-methylazepan-2-one | CN1CCCCCC1=O | Nitrate |
| 2-ethylsulfanylethanol | CCSCCO | Alcohol |
| methyl 3-(3-methoxy-3-oxopropyl)sulfanylpropanoate | COC(=O)CCSCCC(=O)OC | Multiple |
| thiophene-2-carbaldehyde | O=Cc1cccs1 | Aldehyde |
| 1-thiophen-2-ylethanone | CC(=O)c1cccs1 | Keton |
| thiolane 1-oxide | O=S1CCCC1 | Aliphatic |
| oxathiolane 2,2-dioxide | O=S1(=O)CCCO1 | Aliphatic |
| 1,3,2-dioxathiolane 2-oxide | O=S1OCCO1 | Aliphatic |
| 1-propylsulfinylpropane | CCCS(=O)CCC | Aliphatic |
| 2-ethenylthiolane 1,1-dioxide | C=CC1CCCS1(=O)=O | Aliphatic |
| 4-methyl-1,3-thiazol-2-amine | Cc1csc(N)n1 | Nitrate |
| 2-aminobenzenethiol | Nc1ccccc1S | Nitrate |
| 1,3-diacetyloxypropan-2-yl acetate | CC(=O)OCC(COC(C)=O)OC(C)=O | Multiple |
| 2,3-dihydroxypropyl hexadecanoate | CCCCCCCCCCCCCCCC(=O)OCC(O)CO | Multiple |
| (3-hexadecanoyloxy-2-hydroxypropyl) hexadecanoate | CCCCCCCCCCCCCCCC (=O)OCC(O)COC(=O)CCCCC CCCCCCCCCC | Multiple |
| 1,3-di(hexadecanoyloxy)propan-2-yl hexadecanoate | CCCCCCCCCCCCCCCC(=O)OCC (COC(=O)CCCCCCCCCCCCCCC)OC (=O)CCCCCCCCCCCCCCC | Multiple |
| decanoic acid | CCCCCCCCCC(=O)O | Carboxyl |
| tetradecanoic acid | CCCCCCCCCCCCCC(=O)O | Carboxyl |
| octadec-9-enoic acid | CCCCCCCCC=CCCCCCCCC(=O)O | Carboxyl |
| octadecanoic acid | CCCCCCCCCCCCCCCCCC(=O)O | Carboxyl |

| | | |
|---|---|---|
| octadeca-9,12-dienoic acid | CCCCCC=CCC=CCCCCCCCC(=O)O | Carboxyl |
| octadeca-9,12,15-trienoic acid | CCC=CCC=CCC=CCCCCCCCC(=O)O | Carboxyl |
| 1,4,7,10,13,16-hexaoxacyclooctadecane | C1COCCOCCOCCOCCOCCO1 | Ether |
| malononitrile | N#CCC#N | Nitrate |
| 1,2-dicyanoethane | N#CCCC#N | Nitrate |
| glutaronitrile | N#CCCCC#N | Nitrate |
| 2,4-dicyano-1-butene | C=C(C#N)CCC#N | Nitrate |
| NA | N#CCCCCCC#N | Nitrate |
| NA | N#CCCCCCCC#N | Nitrate |
| heptanonitril | CCCCCCC#N | Nitrate |
| octanonitril | CCCCCCCC#N | Nitrate |
| nonanonitril | CCCCCCCCC#N | Nitrate |
| 2,5-dihydrothiophene 1,1-dioxide | O=S1(=O)CC=CC1 | Aliphatic |
| 3-methylthiolane 1,1-dioxide | CC1CCS(=O)(=O)C1 | Aliphatic |
| 2,4-dimethylthiolane 1,1-dioxide | CC1CC(C)S(=O)(=O)C1 | Aliphatic |
| 1,1-dioxothiolan-3-amine | NC1CCS(=O)(=O)C1 | Nitrate |
| 1,3-dioxolan-2-one | O=C1OCCO1 | Ether |
| NA | N#CCCO | Multiple |
| phenylmethanamine | NCc1ccccc1 | Nitrate |
| 2,2-dichloroacetic acid | O=C(O)C(Cl)Cl | Multiple |
| 2-chloroethanol | OCCCl | Multiple |
| dichloro-dioctylstannane | CCCCCCCC[Sn](Cl)(Cl)CCCCCCCC | Halogene |
| 2-hydroxypropanoic acid | CC(O)C(=O)O | Multiple |
| cyclohexylcyclohexane | C1CCC(C2CCCCC2)CC1 | Aliphatic |
| cyclohexylbenzene | c1ccc(C2CCCCC2)cc1 | Aromat |
| 2,6,10,15,19,23-hexamethyl-2,6,10,14,18,22-tetracosahexaene | CC(C)=CCCC(C)=CCCC(C)=CCCC=C(C)CCC=C(C)CCC=C(C)C | Aliphatic |
| 2-propoxyethanol | CCCOCCO | Multiple |
| 2-propan-2-yloxyethanol | CC(C)OCCO | Multiple |
| 3-decoxythiolane 1,1-dioxide | CCCCCCCCCCOC1CCS(=O)(=O)C1 | Ether |
| 1,1-dioxothiolan-3-ol | O=S1(=O)CCC(O)C1 | Alcohol |
| 2-sulfanylethanol | OCCS | Alcohol |
| 2-(2-hydroxyethylsulfanyl)ethanol | OCCSCCO | Alcohol |
| diethyl sulfate | CCOS(=O)(=O)OCC | Aliphatic |
| phenylmethyl acetate | CC(=O)OCc1ccccc1 | Multiple |
| 1-bromo-4-methoxybenzene | COc1ccc(Br)cc1 | Multiple |
| 1-bromonaphthalene | Brc1cccc2ccccc12 | Halogene |
| 1-phenylpropan-1-one | CCC(=O)c1ccccc1 | Keton |
| dipropyl benzene-1,2-dicarboxylate | CCCOC(=O)c1ccccc1C(=O)OCCC | Multiple |

| | | |
|---|---|---|
| dihexyl benzene-1,2-dicarboxylate | CCCCCCOC(=O)c1ccccc1C(=O) OCCCCCC | Multiple |
| dioctyl benzene-1,2-dicarboxylate | CCCCCCCCOC(=O)c1ccccc1C(=O)O CCCCCCCC | Multiple |
| didecyl benzene-1,2-dicarboxylate | CCCCCCCCCCOC(=O) c1ccccc1C(=O)OCCCCCCCCCC | Multiple |
| dipropan-2-yl benzene-1,2-dicarboxylate | CC(C)OC(=O)c1ccccc1C(=O)OC(C)C | Multiple |
| diprop-2-enyl benzene-1,2-dicarboxylate | C=CCOC(=O)c1ccccc1C(=O)OCC=C | Multiple |
| dibutan-2-yl benzene-1,2-dicarboxylate | CCC(C)OC(=O)c1ccccc1C(=O)OC(C)CC | Multiple |
| dihexyl benzene-1,3-dicarboxylate | CCCCCCOC(=O)c1cccc (C(=O)OCCCCCC)c1 | Multiple |
| dihexyl benzene-1,4-dicarboxylate | CCCCCCOC(=O)c1ccc (C(=O)OCCCCCC)cc1 | Multiple |
| (2-butanoyloxyphenyl) butanoate | CCCC(=O)Oc1ccccc1OC(=O)CCC | Multiple |
| o2-(2-butoxy-2-oxoethyl) o1-butyl benzene-1,2-dicarboxylate | CCCCOC(=O)COC(=O) c1ccccc1C(=O)OCCCC | Multiple |
| dihexyl hexanedioate | CCCCCCOC(=O)CCCCC(=O)OCCCCCC | Multiple |
| dihexyl octanedioate | CCCCCCOC(=O)CCCC CCC(=O)OCCCCCC | Multiple |
| 1-ethylsulfinylethane | CCS(=O)CC | Aliphatic |
| 1-methylsulfinylpropane | CCCS(C)=O | Aliphatic |
| 2-ethylsulfinylpropane | CCS(=O)C(C)C | Aliphatic |
| 1-methylsulfonylethane | CCS(C)(=O)=O | Aliphatic |
| dimethyl propanedioate | COC(=O)CC(=O)OC | Multiple |
| phenyl acetate | CC(=O)Oc1ccccc1 | Multiple |
| formamide | NC=O | Nitrate |
| 3,5,5-trimethylcyclohex-2-en-1-one | CC1=CC(=O)CC(C)(C)C1 | Keton |
| dimethyl butanedioate | COC(=O)CCC(=O)OC | Multiple |
| 1,4-oxathiane 4-oxide | O=S1CCOCC1 | Ether |
| 1,2,3-tris(2-cyanoethoxy)propane | N#CCCOCC(COCCC#N)OCCC#N | Multiple |
| 3-{3-(2-cyanoethoxy)-2,2-bis[(2-cyanoethoxy)methyl]propoxy}propanenitrile | N#CCCOCC(COCCC#N)(COCCC #N)COCCC#N | Multiple |
| sebaconitrile | N#CCCCCCCCCC#N | Nitrate |
| 2-[2-[2-(2-hydroxyethoxy)ethoxy] ethoxy]ethanol | OCCOCCOCCOCCO | Multiple |
| 1-bromohexadecane | CCCCCCCCCCCCCCCCBr | Halogene |
| 1-iodohexadecane | CCCCCCCCCCCCCCCCI | Halogene |
| dipropyl 3,4,5,6-tetrachlorobenzene-1,2-dicarboxylate | CCCOC(=O)c1c(Cl)c(Cl)c (Cl)c(Cl)c1C(=O)OCCC | Multiple |

| | | |
|---|---|---|
| 1,1,1,2,2,3,3,4,4-nonafluorodocosane | CCCCCCCCCCCCCCCCCCC(F)(F)C (F)(F)C(F)(F)C(F)(F)F | Halogene |
| 1,1,1,2,2,3,3,4,4,5,5,6,6-tridecafluorodocosane | CCCCCCCCCCCCC CCCC(F)(F)C(F)(F)C(F)(F)C(F)(F) C(F)(F)C(F)(F)F | Halogene |
| 1,1,1,2,2,3,3,4,4,5,5,6,6-tridecafluorooctadecane | CCCCCCCCCCCCC (F)(F)C(F)(F)C(F)(F)C(F) (F)C(F)(F)C(F)(F)F | Halogene |
| 1,1,1,2,2,3,3,4,4,5,5,6,6,7,7,8,8-heptadecafluoroicosane | CCCCCCCCCCCCC (F)(F)C(F)(F)C(F)(F)C(F)(F)C(F)(F)C (F)(F)C(F)(F)C(F)(F)F | Halogene |
| 2-[2-(bis(2-hydroxyethyl)amino)ethyl-(2-hydroxyethyl)amino]ethanol | OCCN(CCO)CCN(CCO)CCO | Multiple |
| n'-(2-aminoethyl)-n-[2-(2-aminoethylamino)ethyl]ethane-1,2-diamine | NCCNCCNCCNCCN | Nitrate |
| tetradecanedinitrile | N#CCCCCCCCCCCCCC#N | Nitrate |
| docosan-1-ol | CCCCCCCCCCCCCCCCCCCCCCO | Alcohol |
| icos-1-ene | C=CCCCCCCCCCCCCCCCCCC | Aliphatic |
| ethyl octanoate | CCCCCCCC(=O)OCC | Multiple |
| pentadecane | CCCCCCCCCCCCCCC | Aliphatic |
| n,n-dibutylbenzamide | CCCCN(CCCC)C(=O)c1ccccc1 | Nitrate |
| methoxyethane | CCOC | Ether |
| methyl 2-methylprop-2-enoate | C=C(C)C(=O)OC | Multiple |
| 2-butene | CC=CC | Aliphatic |
| tetraethylsilane | CC[Si](CC)(CC)CC | Multiple |
| 2-tert-butylperoxy-2-methylpropane | CC(C)(C)OOC(C)(C)C | Aliphatic |
| 4-methylpent-3-en-2-one | CC(=O)C=C(C)C | Keton |
| diethyl carbonate | CCOC(=O)OCC | Ether |
| n-methoxypropan-2-imine | CON=C(C)C | Nitrate |
| 2-(2-aminoethylamino)ethanol | NCCNCCO | Multiple |
| 1,2-dibromopropane | CC(Br)CBr | Halogene |
| n-methylaniline | CNc1ccccc1 | Nitrate |
| n-ethylethane-1,2-diamine | CCNCCN | Nitrate |
| 1-methoxybutane | CCCCOC | Ether |
| 3-methylbutyl acetate | CC(=O)OCCC(C)C | Multiple |
| crotonaldehyde | CC=CC=O | Aldehyde |
| 2-methylpropyl acetate | CC(=O)OCC(C)C | Multiple |
| pyrrolidine | C1CCNC1 | Nitrate |
| propyl butanoate | CCCOC(=O)CCC | Multiple |
| 1,1-diethoxyethane | CCOC(C)OCC | Ether |

| | | |
|---|---|---|
| methyl 2-hydroxypropanoate | COC(=O)C(C)O | Multiple |
| ethyl 2-hydroxypropanoate | CCOC(=O)C(C)O | Multiple |
| ethyl 2-methylpropanoate | CCOC(=O)C(C)C | Multiple |
| 5-(hydroxymethyl)furan-2-carbaldehyde | O=Cc1ccc(CO)o1 | Multiple |
| pentanoic acid | CCCCC(=O)O | Carboxyl |
| 1-methyl-4-propan-2-ylbenzene | Cc1ccc(C(C)C)cc1 | Aromat |
| 3-chloroaniline | Nc1cccc(Cl)c1 | Multiple |
| 4-chloroaniline | Nc1ccc(Cl)cc1 | Multiple |
| 3,4-dichloroaniline | Nc1ccc(Cl)c(Cl)c1 | Multiple |
| 2-methylpropanoic acid | CC(C)C(=O)O | Carboxyl |
| 5-chloropentan-2-one | CC(=O)CCCCl | Multiple |
| 1-isocyanato-4-[(4-isocyanatophenyl)methyl]benzene | O=C=Nc1ccc(Cc2ccc(N=C=O)cc2)cc1 | Nitrate |
| chlorocyclohexane | ClC1CCCCC1 | Halogene |
| 1,2-dichloro-4-isocyanatobenzene | O=C=Nc1ccc(Cl)c(Cl)c1 | Multiple |
| 2-methylpropylbenzene | CC(C)Cc1ccccc1 | Aromat |
| 2-chloroacetic acid | O=C(O)CCl | Multiple |
| 4-methylpentan-2-ol | CC(C)CC(C)O | Alcohol |
| n,n-diethylformamide | CCN(C=O)CC | Nitrate |
| n-methylcyclohexanamine | CNC1CCCCC1 | Nitrate |
| ethoxymethoxyethane | CCOCOCC | Ether |
| 1,4-difluorobenzene | Fc1ccc(F)cc1 | Halogene |
| 1,2,3,4,5-pentafluorobenzene | Fc1cc(F)c(F)c(F)c1F | Halogene |
| methyl 2,2,3,3,4,4,4-heptafluorobutanoate | COC(=O)C(F)(F)C(F)(F)C(F)(F)F | Multiple |
| butyl 2-methylprop-2-enoate | C=C(C)C(=O)OCCCC | Multiple |
| 2-chlorophenol | Oc1ccccc1Cl | Multiple |
| heptan-3-one | CCCCC(=O)CC | Keton |
| oct-1-en-4-one | C=CCC(=O)CCCC | Keton |
| 1,1,1,2,3,3-hexafluoro-3-(2,2,2-trifluoroethoxy)propane | FC(C(F)(F)F)C(F)(F)OCC(F)(F)F | Multiple |
| 2-fluoropropane | CC(C)F | Halogene |
| 1,1,1,2,2,3,3,4,4,4-decafluorobutane | FC(F)(F)C(F)(F)C(F)(F)C(F)(F)F | Halogene |
| 2-methylprop-2-enoic acid | C=C(C)C(=O)O | Carboxyl |
| 1-ethoxypropane | CCCOCC | Ether |
| 1-hexoxyhexane | CCCCCCOCCCCCC | Ether |
| 1,3-benzothiazole | c1ccc2scnc2c1 | Nitrate |
| azepane | C1CCCNCC1 | Nitrate |
| 3-ethylpentan-3-ol | CCC(O)(CC)CC | Alcohol |
| 1-methylpiperidine | CN1CCCCC1 | Nitrate |
| 3-methylheptan-3-ol | CCCCC(C)(O)CC | Alcohol |

| | | |
|---|---|---|
| thionyl dichloride | O=S(Cl)Cl | Halogene |
| 3-methylthiophene | Cc1ccsc1 | Aromat |
| 1,2,3-trimethylbenzene | Cc1cccc(C)c1C | Aromat |
| 1h-indole | c1ccc2[nH]ccc2c1 | Nitrate |
| 2-methylprop-1-ene | C=C(C)C | Aliphatic |
| 4,4-dimethyl-1,3-dioxane | CC1(C)CCOCO1 | Ether |
| 1,2-bis(2-methoxyethoxy)ethane | COCCOCCOCCOC | Ether |
| 2,4-diisocyanato-1-methylbenzene | Cc1ccc(N=C=O)cc1N=C=O | Nitrate |
| butyl propanoate | CCCCOC(=O)CC | Multiple |
| 3-chloroprop-1-ene | C=CCCl | Halogene |
| propyl propanoate | CCCOC(=O)CC | Multiple |
| acetyloxymethyl acetate | CC(=O)OCOC(C)=O | Multiple |
| ethenyl butanoate | C=COC(=O)CCC | Multiple |
| [dimethyl-(trimethylsilylamino)silyl]methane | C[Si](C)(C)N[Si](C)(C)C | Other |
| 1-chloro-1-fluoroethane | CC(F)Cl | Halogene |
| naphthalene | c1ccc2ccccc2c1 | Aromat |
| octan-2-ol | CCCCCCC(C)O | Alcohol |
| 1,2-diethoxyethane | CCOCCOCC | Ether |
| 2-butyloxirane | CCCCC1CO1 | Ether |
| 1,1-dimethylhydrazine | CN(C)N | Nitrate |
| 2,4-dimethylpentan-3-one | CC(C)C(=O)C(C)C | Keton |
| ethyldisulfanylethane | CCSSCC | Aliphatic |
| 2-methylbut-1-ene | C=C(C)CC | Aliphatic |
| undecan-1-ol | CCCCCCCCCCCO | Alcohol |
| 1,1-dimethoxyethane | COC(C)OC | Ether |
| trimethoxyborane | COB(OC)OC | Aliphatic |
| nonan-5-one | CCCCC(=O)CCCC | Keton |
| methoxycyclopentane | COC1CCCC1 | Ether |
| 2-hex-5-enyloxirane | C=CCCCCC1CO1 | Ether |
| 1,4-dichlorobuta-1,3-diyne | ClCCCCCl | Halogene |
| 2-(2-hydroxyethylamino)ethanol | OCCNCCO | Multiple |
| pentane-1-thiol | CCCCCS | Aliphatic |
| 1-phenylethanol | CC(O)c1ccccc1 | Alcohol |
| molecular chlorine | ClCl | Halogene |
| trichloroborane | ClB(Cl)Cl | Halogene |
| 1h-pyrrole | c1cc[nH]c1 | Nitrate |
| chloromethane | CCl | Halogene |
| fluoroform | FC(F)F | Halogene |
| prop-2-enal | C=CC=O | Aldehyde |
| ethyl hexanoate | CCCCCC(=O)OCC | Multiple |

| | | |
|---|---|---|
| ethyl tetradecanoate | CCCCCCCCCCCCCC(=O)OCC | Multiple |
| ethyl decanoate | CCCCCCCCCC(=O)OCC | Multiple |
| 9h-fluorene | c1ccc2c(c1)Cc1ccccc1-2 | Aromat |
| dibenzofuran | c1ccc2c(c1)oc1ccccc12 | Aromat |
| 1,1,1,2,2,3,4,5,5,5-decafluoropentane | FC(C(F)C(F)(F)C(F)(F)F)C(F)(F)F | Halogene |
| 1-buten-3-yne | C#CC=C | Aliphatic |
| 2-methylaniline | Cc1ccccc1N | Nitrate |
| methyl-bis(trimethylsilyloxy)silicon | C[Si](O[Si](C)(C)C)O[Si](C)(C)C | Multiple |
| trichloroarsane | Cl[As](Cl)Cl | Halogene |
| 1,1-dichloro-1-fluoroethane | CC(F)(Cl)Cl | Halogene |
| 1,1,1,2,2,3,3,4,5,5,5-undecafluoro-4-(trifluoromethyl)pentane | FC(F)(F)C(F)(F)C(F)(F)C(F)(C(F)(F)F)C(F)(F)F | Halogene |
| hydrogen peroxide | OO | Multiple |
| azepan-2-one | O=C1CCCCCN1 | Nitrate |
| 2,4-dimethylpyridine | Cc1ccnc(C)c1 | Nitrate |
| propan-2-amine | CC(C)N | Nitrate |
| hexane-1,6-diamine | NCCCCCCN | Nitrate |
| 2-methyl-1,3-dioxolane | CC1OCCO1 | Ether |
| 2-amino-2-methylpropan-1-ol | CC(C)(N)CO | Multiple |
| 2-diethylaminoethanol | CCN(CC)CCO | Multiple |
| methyl 2-hydroxy-2-methylpropanoate | COC(=O)C(C)(C)O | Multiple |
| 2-methylpentane-1,5-diamine | CC(CN)CCCN | Nitrate |
| n-(2-aminoethyl)ethane-1,2-diamine | NCCNCCN | Nitrate |
| cyclopropanecarbonitrile | N#CC1CC1 | Nitrate |
| n-(3-aminopropyl)propane-1,3-diamine | NCCCNCCCN | Nitrate |
| n-methylpropane-1,3-diamine | CNCCCN | Nitrate |
| 3-dimethylaminopropan-1-ol | CN(C)CCCO | Multiple |
| 2-(propan-2-ylamino)ethanol | CC(C)NCCO | Multiple |
| pentane-1,3-diamine | CCC(N)CCN | Nitrate |
| chloro-trimethylsilane | C[Si](C)(C)Cl | Other |
| dichloro-dimethylsilane | C[Si](C)(Cl)Cl | Other |
| ethyl 2,2,2-trichloroacetate | CCOC(=O)C(Cl)(Cl)Cl | Multiple |
| hexafluorotungsten | F[W](F)(F)(F)(F)F | Other |
| butanoyl butanoate | CCCC(=O)OC(=O)CCC | Multiple |
| 1,1,2,3,3,3-hexafluoroprop-1-ene | FC(F)=C(F)C(F)(F)F | Halogene |
| dichloro-fluoromethane | FC(Cl)Cl | Halogene |
| bromo-trifluoromethane | FC(F)(F)Br | Halogene |
| 1,1,1,2,2,2-hexafluoroethane | FC(F)(F)C(F)(F)F | Halogene |
| 1,1,1,2,2,3,3,3-octafluoropropane | FC(F)(F)C(F)(F)C(F)(F)F | Halogene |
| trichloro-fluoromethane | FC(Cl)(Cl)Cl | Halogene |

| | | |
|---|---|---|
| n-cyclohexylidenehydroxylamine | ON=C1CCCCC1 | Nitrate |
| cyclohexyl formate | O=COC1CCCCC1 | Ether |
| methyl octadecanoate | CCCCCCCCCCCCCCCCCC(=O)OC | Multiple |
| octanoic acid | CCCCCCCC(=O)O | Carboxyl |
| heptanoic acid | CCCCCCC(=O)O | Carboxyl |
| ethyl 3-ethoxyprop-2-enoate | CCOC=CC(=O)OCC | Multiple |
| 2-(2-hexoxyethoxy)ethanol | CCCCCCOCCOCCO | Multiple |
| dimethyl benzene-1,3-dicarboxylate | COC(=O)c1cccc(C(=O)OC)c1 | Multiple |
| furan-2,5-dione | O=C1C=CC(=O)O1 | Multiple |
| 1,3-dibromopropane | BrCCCBr | Halogene |
| 3,4-dimethylphenol | Cc1ccc(O)cc1C | Alcohol |
| tetrafluoromethane | FC(F)(F)F | Halogene |
| phenanthrene | c1ccc2c(c1)ccc1ccccc12 | Aromat |
| 1-ethyl-2-methylbenzene | CCc1ccccc1C | Aromat |
| 3,7,7-trimethylbicyclo[4.1.0]hept-3-ene | CC1=CCC2C(C1)C2(C)C | Aliphatic |
| 1,1,1,7-tetrachloroheptane | ClCCCCCCC(Cl)(Cl)Cl | Halogene |
| 1-chloro-4-methylbenzene | Cc1ccc(Cl)cc1 | Halogene |
| 6-methylhept-5-en-2-one | CC(=O)CCC=C(C)C | Keton |
| 1-pentoxypentane | CCCCCOCCCCC | Ether |
| bromo-chloro-difluoromethane | FC(F)(Cl)Br | Halogene |
| 1-propan-2-yl-4-[(4-propan-2-ylphenyl)methyl]benzene | CC(C)c1ccc(Cc2ccc(C(C)C)cc2)cc1 | Aromat |
| 2,2-dimethyloxirane | CC1(C)CO1 | Ether |
| 3,7-dimethyloctan-3-ol | CCC(C)(O)CCCC(C)C | Alcohol |
| pentafluoro-lambda5-bromane | FBr(F)(F)(F)F | Other |
| pentafluoro-lambda5-iodane | FI(F)(F)(F)F | Other |
| 1-methoxypropan-2-yl acetate | COCC(C)OC(C)=O | Multiple |
| dichlorozinc | Cl[Zn]Cl | Halogene |
| sodium nitrite | O=N[O-].[Na+] | Other |
| triethylstibane | CC[Sb](CC)CC | Multiple |
| 2-chloro-1,1,1,2-tetrafluoropropane | CC(F)(Cl)C(F)(F)F | Halogene |

# References

T. Brouwer, S. R. Kersten, G. Bargeman, and B. Schuur. trends in solvent impact on infinite dilution activity coefficients of solutes reviewed and visualized using an algorithm to support selection of solvents for greener fluid separations. *Separation and Purification Technology*, 272:118727, 2021. ISSN 13835866. doi: 10.1016/j.seppur.2021.118727.

Dortmund Datenbank, 2022. URL `http://www.ddbst.com/`.

B. Winter, C. Winter, J. Schilling, and A. Bardow. A smile is all you need: Predicting limiting activity coefficients from SMILES with natural language processing, 2022. URL `https://arxiv.org/pdf/2206.07048`.
